# Supplementary material for: ReCaLL: Membership Inference via Relative Conditional Log-Likelihoods
Source: arXiv:2406.15968 source file (2025-05-23)
Supplement: Supplementary file 1 [file temporal_dataset.tex]

\begin{table}[h!]
\centering
\begin{tabular}{ccccccc}
\toprule
\textbf{\# Params} & \textbf{Loss} & \textbf{Ref} & \textbf{Zlib} & \textbf{Min-K\%} & \textbf{Min-K\%++} & \textbf{ReCaLL} \\
\midrule
160M  & 64.0  & 62.2  & 54.4  & 64.8  & 63.1  & 71.9 \\
1.4B  & 66.1  & 68.7  & 58.4  & 68.7  & 72.6  & 73.2 \\
2.8B  & 67.4  & 75.4  & 59.9  & 70.6  & 74.7  & 76.1 \\
6.9B  & 69.2  & 78.8  & 62.5  & 73.3  & 79.2  & 80.1 \\
12B   & 70.8  & 79.1  & 64.3  & 75.4  & 80.7  & 82.1 \\
\bottomrule
\end{tabular}
\caption{Temporal arXiv Benchmark}
\end{table}

\begin{table}[h!]
\centering
\begin{tabular}{ccccccc}
\toprule
\textbf{\# Params} & \textbf{Loss} & \textbf{Ref} & \textbf{Zlib} & \textbf{Min-K\%} & \textbf{Min-K\%++} & \textbf{ReCaLL} \\
\midrule
160M  & 61.9  & 62.9  & 59.8  & 60.9  & 61.1  & 67.9 \\
1.4B  & 65.1  & 65.4  & 63.0  & 64.6  & 59.7  & 72.3 \\
2.8B  & 66.2  & 67.7  & 64.1  & 65.9  & 60.4  & 72.6 \\
6.9B  & 67.5  & 69.0  & 65.2  & 67.8  & 62.8  & 75.1 \\
12B   & 68.2  & 70.9  & 66.0  & 68.9  & 64.8  & 76.0 \\
\bottomrule
\end{tabular}
\caption{Temporal arXiv Benchmark - Another Dataset}
\end{table}
